# Supplementary material for: CLIP Guided Image-perceptive Prompt Learning for Image Enhancement
Source: arXiv:2311.03943 source file (2023-11-22)
Supplement: Supplementary file 1 [file supp.tex]

\clearpage
\section{The Experiments on the Resolution of 512}
We also evaluate the performance on three datasets: Jung~\cite{jung2018water}, Kligler~\cite{kligler2018document}, and the proposed SD7K, in a relatively low resolution of 512 $\times$ 512 where the divisions between training and testing are shown in Table~\ref{table:eval}. We train each dataset separately to satisfy the settings of the previous works. The batch size is set to 1 for the other two datasets due to the limited samples. 

\input{tabletex/6_exp/dataset}

 We give the quantitative evaluation in Table~\ref{table:low} and the visual results are available in Figure~\ref{fig:lowres} and Figure~\ref{fig:lowres0}.
As shown in Table~\ref{table:low}, our proposed FSENet outperforms all other methods under the low-resolution data setting. In the Figure~\ref{fig:lowres} and Figure~\ref{fig:lowres0}, we can clearly observe that Wang \etal~\cite{Wang2020ShadowRO}, SP+M+I Net~\cite{le2021physics}, SG-ShadowNet~\cite{wan2022style} and ShadowFormer~\cite{guo2023shadowformer} exhibit the phenomenon of incomplete shadow removal. Meanwhile, \cite{Wang2020ShadowRO} shows a large difference from the target in white balance. Despite BEDSR-Net~\cite{lin2020bedsr} performing relatively well in both white balance and shadow removal, a close examination of the finer details reveals that BEDSR-Net yields blurry results with missing texture details. Simultaneously, BEDSR-Net fails in Figure~\ref{fig:lowres0} in terms of shadow removal. In comparison, our result achieves the best performance in white balance, shadow removal, and detail restoration.

\section{More High-Resolution Results on SD7K}
We give more visual comparisons on the high-resolution inputs in Figure~\ref{fig:highres_supp}. The results in the first two rows come from Kligler dataset, and the results in the last two rows come from SD7K. It can be observed that the shadow removal results from Jung \etal~\cite{jung2018water} are unstable, and the white balance often differs from the target. Meanwhile, shadow removal with MaskShadowGAN~\cite{hu2019mask} is always incomplete, with the original shadow regions prone to leaving stains and causing texts to become unreadable. In contrast, our method performs relatively well in both white balancing and shadow removal.

\subsection{The Detailed Structure of DFE and TAA Blocks}
In Sec. 4 of the main paper, we show the introduction of the TAA and DFE by text description, here, we give a detailed network structure to better understand our method as shown in Figure~\ref{fig:dfe_taa}.

\input{figtex/dfe}

\input{figtex/6_exp/lowres}
\input{figtex/6_exp/lowres0}
\input{tabletex/6_exp/low}

\input{figtex/6_exp/highres_supp}
